# Supplementary material for: Combined Robust and Stochastic Model Predictive Control for Models of Different Granularity
Source: arXiv:2003.06652 source file (2021-05-14)
Supplement: Supplementary file 1 [file appendixa.tex]

% \section{Appendix A}
% \label{sec:appendixa}

% Appendixes, if needed, appear before the acknowledgment.
